# Supplementary material for: Automatic Recognition of Food Ingestion Environment from the AIM-2 Wearable Sensor
Source: arXiv:2405.07827 source file (2024-05-13)
Supplement: Supplementary file 1 [file X_suppl.tex]

\clearpage
\setcounter{page}{1}
\maketitlesupplementary

\section{Data Processing}

We collected experimental data from thirty volunteer participants (65\% males and 35\% females, aged 18 to 39 years old). The University of Alabama institutional review board approved the study, and participants were compensated for their participation. The subjects represented four races, non-Hispanic, African American, Asian, and Hispanic.

To classify the environment of food consumption, ASA24 defines fourteen ingestion environments including home, fast-food restaurant, other restaurants, cafeteria, bar or tavern, work, car, sports or entertainment venue, someplace else, school cafeteria (child version only), school, not in the cafeteria (child version only), don’t know, and outdoor/picnic.

Out of the 14 ingestion environments defined by ASA24, the following are dropped out in our study: 1) School cafeteria and school, not in the cafeteria, since the study did not involve school children and none of the participants reported on those classes; 2) Fast-food restaurants, bar, and tavern as none of the participants reported on those classes; 3) Sports or entertainment venue, and outdoors, as only one instance was reported for these categories.

In total, the participants consumed 89 meals in different environments. We found that 17 (19\%) entries related to ingestion environments were incorrectly reported by the participants based on examining the capture images, which is consistent with our previous statement in the introduction. After evaluating why this may have happened, it appears that participants often got confused with the question in ASA24 about the source of the food versus another question about the environment in which the foods were consumed, for example, fast-food takeout consumed at home based on captured images was reported as a restaurant in ASA24 instead of at home. Furthermore, few participants reported unknown locations of food consumption. 

Developing a methodology based on incorrect assessment would be undesirable. Therefore, we corrected the falsely reported self-assessment data by using Giacchi's self-reporting data correction approach. We performed an expert review of the entire dataset. We reviewed each image sequence during the expert review, including images before, after, and during the eating episode to determine the actual ingestion environment. After this, we made corrections to the self-reported ingestion environment.

Three instances of eating at other restaurants were reported, therefore, we combined restaurants and cafeterias as one group (restaurant). Thus, the total eating episodes were relabeled to 89 eating episodes representing four ingestion environments consisting of 64 at home, 13 at a restaurant, 10 at work, and 2 in a vehicle/car. These four ingestion environments amounted to 5,351 images representing the temporal image sequence of the eating episodes for all 89 meals. Note that each sequence corresponds to one meal with one ingestion environment and each sequence can have different numbers of images depending on the eating duration.

\begin{figure*}[t]
\centering
\includegraphics[width=0.95\textwidth]{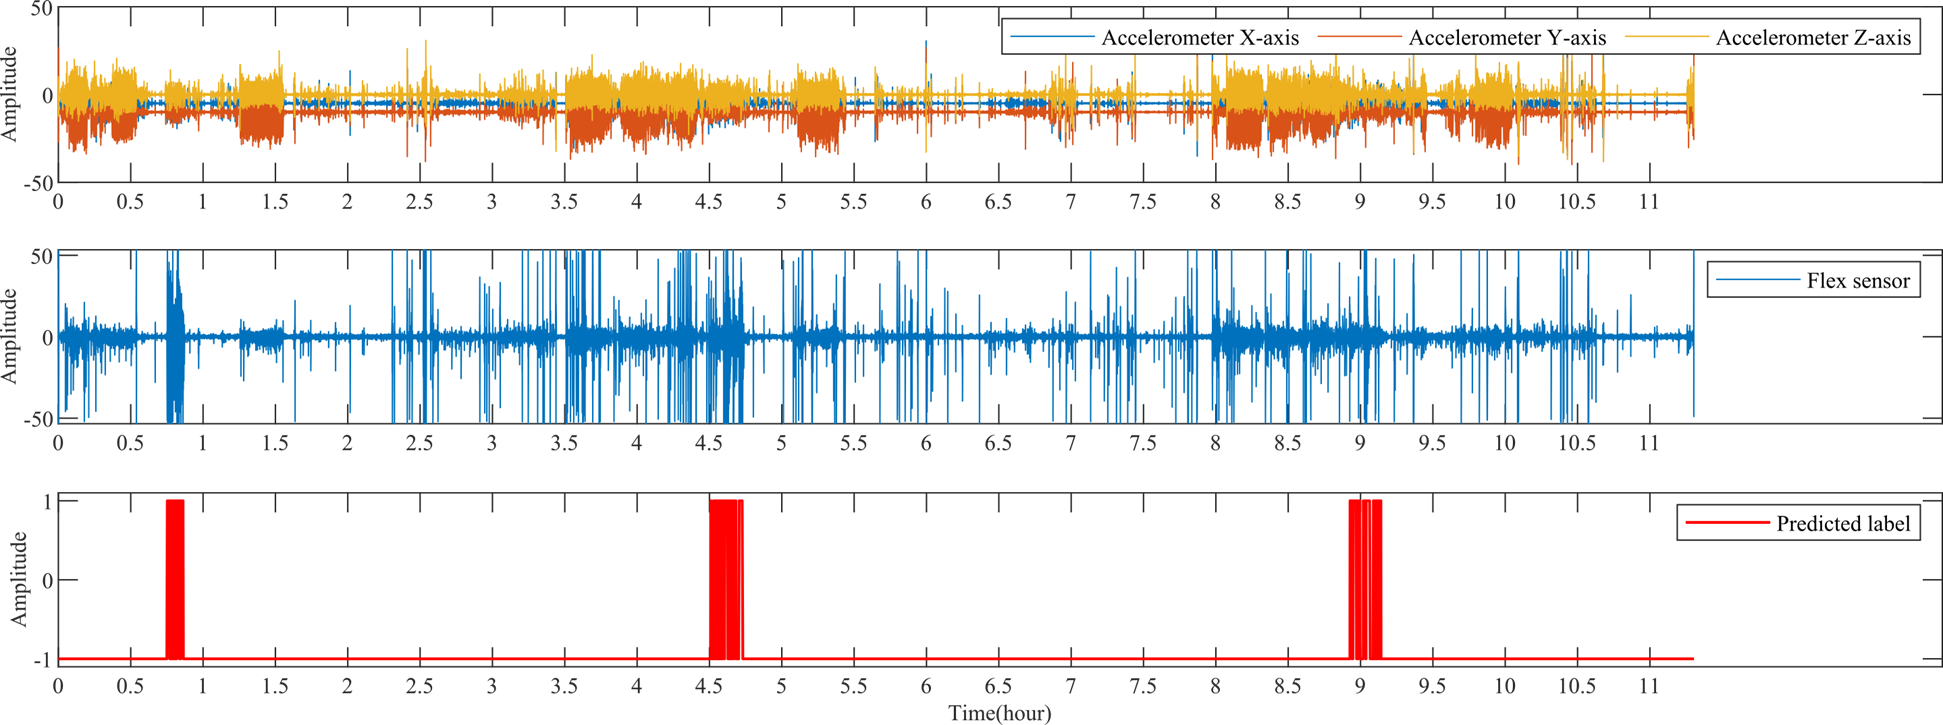} 
\caption{Description of food intake detection using accelerometer and bend sensor data.}
\label{fig: food intake detection}
\end{figure*}
\section{Eating Period Detection}

In the mode of operation used for this study, AIM-2 captured images continuously throughout the day. To characterize the ingestion environment, the eating episodes need to be detected and separated. Here a combination of accelerometer and flexible sensor signals were used to detect the beginning and the end of an eating episode. The flexible sensor captured information from the movement of the temporal muscle. 

The accelerometer captures information on head movement (see Fig.~\ref{fig: food intake detection}). Both sensor signals from the accelerometer and the flexible sensor were preprocessed to remove noise and perform normalization. Upon preprocessing, the signals were divided into 10s non-overlapping epochs, and a combination of 38 features was extracted for each of the sensor signals. The features were used to perform the detection of eating and to determine the start time and end time of eating episodes

\begin{table}[]
\caption{Data Partition Details}
\centering
\resizebox{0.475\textwidth}{!}{
\begin{tabular}{c|cccc|c}
\hline
\multirow{2}{*}{Partition} & \multicolumn{4}{c|}{Number of Sequences}                                                                 & \multirow{2}{*}{Images} \\ \cline{2-5}
                           & \multicolumn{1}{c|}{Vehicle} & \multicolumn{1}{c|}{Home} & \multicolumn{1}{c|}{Restaurant} & Workplace &                               \\ \hline
1                          & \multicolumn{1}{c|}{1}       & \multicolumn{1}{c|}{11}   & \multicolumn{1}{c|}{3}          & 4         & 908                           \\ \hline
2                          & \multicolumn{1}{c|}{0}       & \multicolumn{1}{c|}{18}   & \multicolumn{1}{c|}{0}          & 0         & 796                           \\ \hline
3                          & \multicolumn{1}{c|}{0}       & \multicolumn{1}{c|}{13}   & \multicolumn{1}{c|}{2}          & 3         & 916                           \\ \hline
4                          & \multicolumn{1}{c|}{0}       & \multicolumn{1}{c|}{11}   & \multicolumn{1}{c|}{5}          & 2         & 1,327                          \\ \hline
5                          & \multicolumn{1}{c|}{1}       & \multicolumn{1}{c|}{11}   & \multicolumn{1}{c|}{0}          & 4         & 1,404                          \\ \hline
\end{tabular}
}
\label{table:partition detail}
\end{table}
\section{K-fold Partition}
In our experiments, we separate the training and testing partition at the sequence level, which means we select all images corresponding to one meal as one sequence and then select 20\% of sequences as the testing set and the rest 80\% as the training set. This manner of separation is important since by doing sequence-level partitioning, we can ensure that data in the testing partition are unseen data, which better illustrates our models' generalization ability.
 
In each step of cross-validation, we use four partitions as the training set and the remaining partition as the testing set. The partitions are fixed in all experiments, the details of each partition are presented in Table~\ref{table:partition detail}. Note that the total number of images in each partition does not need to be the same since the partition is at the sequence-level and each sequence may contain a different number of images. 

\section{Metrics}
\label{sec:rationale}
\textbf{Macro-Average precision:}
We first calculate the precision for each class and then calculate the arithmetic mean among all the classes, as defined in (\ref{eq:precision}) and (\ref{eq:macro-precision}).
\begin{align}
    \label{eq:precision}
    \text{precision}_i &= \frac{TP_i}{TP_i+FP_i}
    \\
    \label{eq:macro-precision}
    \text{macro-precision} &= \frac{1}{n} \sum_{i=1}^{n} \text{precision}_i,
\end{align}
where $i$ is the index of class, $TP_i$ and $FP_i$ are the corresponding true-positive rate and false-positive rate for class $i$.

\textbf{Macro-Average recall:}
Similar to Macro-Average precision, Macro-Average recall is the arithmetic mean of all recalls for each class defined as (\ref{eq:recall}) and (\ref{eq:macro-recall}).

\begin{equation}
\label{eq:recall}
    \text{recall}_i = \frac{TP_i}{TP_i+FN_i}
\end{equation}
\begin{equation}
\label{eq:macro-recall}
    \text{macro-recall} = \frac{1}{n} \sum_{i=1}^{n} \text{recall}_i
\end{equation}
where $i$ is the index of class, $TP_i$ and $FN_i$ are the corresponding true-positive rate and false-negative rate for class $i$.

\textbf{Macro-Average F1 score:}
The Macro-Average F1 score is calculated using Macro-Average precision and Macro-Average recall:
\begin{equation}
\label{eq:F1}
    \text{macro-F1} = 2*\frac{\text{macro-precision} * \text{macro-recall}}{\text{marco-precision} + \text{marco-recall}}
\end{equation}
